# Supplementary material for: Service Differentiation and Fair Sharing in Distributed Quantum Computing
Source: arXiv:2301.03977 source file (2023-01-10)
Supplement: Supplementary file 1 [file appendix.tex]

\section*{Appendix A}\label{sec:appendix:a}

The fidelity of the end-to-end entangled qubits mediated by $L$ intermediate
repeaters is~\cite{briegel_quantum_1998}:

\begin{equation}
    \label{eq:fidelity:generic}
    F' = \frac{1}{4} +
    \frac{3}{4} \left( \frac{p_1^2 p_2 \left( 4 \eta^2 - 1 \right)}{3}\right)^L
    \left( \frac{4\bar{F}-1}{3} \right)^{L+1},
\end{equation}

where $p_1$ is the reliability of one-qubit operations, $p_2$ that
of two-qubit operations, and $\eta$ is the probability of the
measurement giving the wrong result.
In the paper we assume for simplicity that $p_1 = p_2 = \eta = 1$, i.e.,
that all operations to carry out the swapping of qubits are perfect, therefore
\req{fidelity:generic} reduces to \req{fidelity:perfect}.
